# Supplementary material for: Code as Anchor, Memory and Metaphor as Support: Learner Experiences with Multi-View Visualizations
Source: arXiv:2606.19570 source file (2026-06-17)
Supplement: Supplementary file 1 [file 10appendix.tex]

\appendix
\section{Recruitment Emails (Anonymized)}
\label{recruit-email}

\begin{tcolorbox}[colback=gray!5,colframe=black!40,arc=3mm,boxrule=0.5pt]
\textbf{Subject:} Share Your Thoughts on Programming Tools and Earn a \$30 Gift Card  

\vspace{1em}
Dear [Student Name],  

\vspace{0.5em}
We are conducting a research study to understand how visual analogy programming tools can help students learn programming concepts. As a former [introductory programming course] student, your experiences and feedback would be invaluable to this study!  

\vspace{0.5em}
The study involves a 45--60 minute in-person interview where you will:  
\begin{itemize}
    \item Discuss your experiences with programming tools.  
    \item Share your thoughts on visual representations of programming concepts like functions, conditions, lists, and sorting.  
    \item Help us identify ways to improve these tools for future learners.  
\end{itemize}

As a thank-you, participants will receive a \$30 gift card after completing the interview.  

\vspace{0.5em}
If you’re interested, please reply to this email or fill out [form link] by [deadline, if applicable]. We’ll reach out to schedule a time that works for you.  

\vspace{0.5em}
Thank you for considering this opportunity!  

\vspace{1em}
Best regards,  \\
Researcher Name \\ 
Position/Role \\
Institution Name \\
\end{tcolorbox}

\section{Participant Details}
\label{sec:participant-details}
\input{tables/participants}

\section{Interview Protocol}
\label{sec:protocol}
\begin{tcolorbox}[colback=gray!5,colframe=black!40,arc=3mm,boxrule=0.5pt]

\subsection*{General Guidelines}

\paragraph{Introduction.} 
Explain the purpose of the study, obtain consent, and collect brief demographic information (programming experience, language background, etc.).

\paragraph{Think-Aloud Protocol.} 
Remind participants to verbalize their thoughts as they work through the visual examples. Encourage them to describe what they see, what they think is happening, and any challenges they face.

\paragraph{Observations.} 
Make brief notes on any points of confusion, hesitation, or interesting comments that arise during the tasks.
\end{tcolorbox}

\begin{tcolorbox}[colback=gray!5,colframe=black!40,arc=3mm,boxrule=0.5pt]
\subsection*{Group-Specific Instructions}

\paragraph{Group A.} TOOL LINK REDACTED

\paragraph{Group B.} TOOL LINK REDACTED

\paragraph{Tool Sequence Introduction.} 
Inform the participant: 
\begin{quote}
``Today you will start with Python Tutor/MER tool. Once you complete each task with Python Tutor, you will switch to the MER tool/Python Tutor to complete the next task.''
\end{quote}

\paragraph{During Each Task.} 
Prompt the participant to follow along with the visual example. Ask:
\begin{itemize}
    \item What do you notice in this visual representation?
    \item How is the change in variables or control flow depicted for you?
\end{itemize}

\paragraph{Task-Specific Follow-Up Questions.}
\begin{itemize}
    \item \textbf{Task 1: Functions} --- ``What part of the visualization clarified function scope for you?''
    \item \textbf{Task 2: While Loops} --- ``As you followed the while loop, what visual cues helped you see the progression of the counter?'' ``Were there any parts of the loop’s execution that you felt needed more clarity?''
    \item \textbf{Task 3: Linked List} --- ``What did you observe about how the linked list structure changed after the append operation?''
\end{itemize}

\paragraph{Transition Questions (After Completing the First Tool).}
\begin{itemize}
    \item How would you compare your understanding of the tasks after using Python Tutor?
    \item Are there any aspects you found particularly helpful or limiting in Python Tutor before you switch to the next tool?
\end{itemize}

\paragraph{After the Second Tool (MER Tool).} 
Ask similar follow-up questions, encouraging comparisons:
\begin{itemize}
    \item What differences do you notice between Python Tutor and the MER Tool?
    \item Which tool provided clearer visual cues for you, and why?
    \item Were there any moments in the MER/PT Tool where the visualization significantly changed your understanding of the code?
\end{itemize}
\end{tcolorbox}

\begin{tcolorbox}[colback=gray!5,colframe=black!40,arc=3mm,boxrule=0.5pt]

\subsection*{Post-Task Interview}

\paragraph{Overall Tool Effectiveness.}
\begin{itemize}
    \item Overall, which tool did you find more helpful for understanding the programming concepts? Why?
    \item Were there any specific visual features in one tool that you preferred over the other?
\end{itemize}

\paragraph{Usability and Cognitive Load.}
\begin{itemize}
    \item How easy was it to follow the code execution in each tool?
    \item Did you feel that any of the visualizations were overwhelming or confusing at any point?
\end{itemize}

\paragraph{Suggestions for Improvement.}
\begin{itemize}
    \item If you could improve one aspect of either tool’s visualization, what would it be?
    \item Do you have any suggestions for making the visualizations more intuitive or informative?
\end{itemize}

\paragraph{Final Thoughts.} 
\begin{itemize}
    \item Is there anything else you’d like to share about your experience with these tools?
\end{itemize}
\end{tcolorbox}

\begin{tcolorbox}[colback=gray!5,colframe=black!40,arc=3mm,boxrule=0.5pt]

\subsection*{Closing the Session}

Thank the participant for their time and contributions. Remind them about data confidentiality and any follow-up procedures.  

\end{tcolorbox}

\section{Student Task Questions}
\label{sec:tasks}

\begin{table}[h]
\centering

\begin{tabular}{|p{2.5cm}|p{9.5cm}|p{3cm}|}
\hline
\textbf{Topic} & \textbf{Question} & \textbf{Type} \\
\hline
\multirow{3}{*}{\textbf{Scope}} 
& What is the value of the global variable \texttt{a} after \texttt{my\_add(a, b)} is called? & Tracing \\
\cline{2-3}
& What is the value of the local variable \texttt{a} right before the return statement? & Tracing \\
\cline{2-3}
& Explain why the global variable remains unchanged. & Explaining \\
\hline
\multirow{3}{*}{\textbf{While Loops}} 
& What value will be printed? Trace each step of the loop. & Tracing \\
\cline{2-3}
& Explain in plain English how the while loop searches for the item. What role does the counter play, and how does the loop stop? & Explaining \\
\cline{2-3}
& How would you modify the code so that if the wanted item is not in the list, the program prints ``Item not found'' instead of running indefinitely? & Extending \\
\hline
\multirow{3}{*}{\textbf{Linked Lists}} 
& What are the values of \texttt{data} and \texttt{next} for each node in the list? List them in order. & Tracing \\
\cline{2-3}
& Explain how the append function works when adding a new node, differentiating between an empty list and a populated list. & Explaining \\
\cline{2-3}
& How would you implement a \texttt{find(data)} method, and what would happen if the value does not exist? & Extending \\
\hline
\end{tabular}
\caption{Student task questions organized by topic and type.}
\label{tab:student-task-questions}
\end{table}
\section{Example Images of Student Tasks}
\label{example-images}
\begin{figure}[h]
    \centering
    \includegraphics[width=0.7\textwidth]{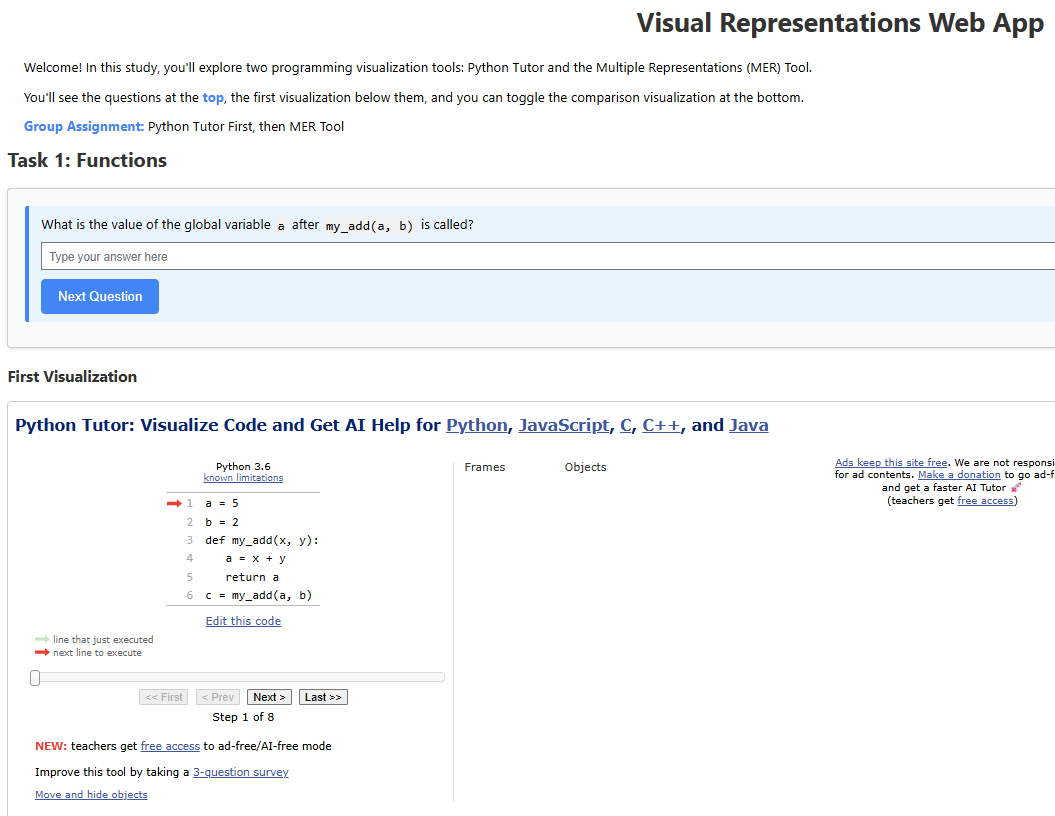}
    \caption{Python Tutor visualization}
    \label{fig:viz1}
\end{figure}

\begin{figure}[h]
    \centering
    \includegraphics[width=0.7\textwidth]{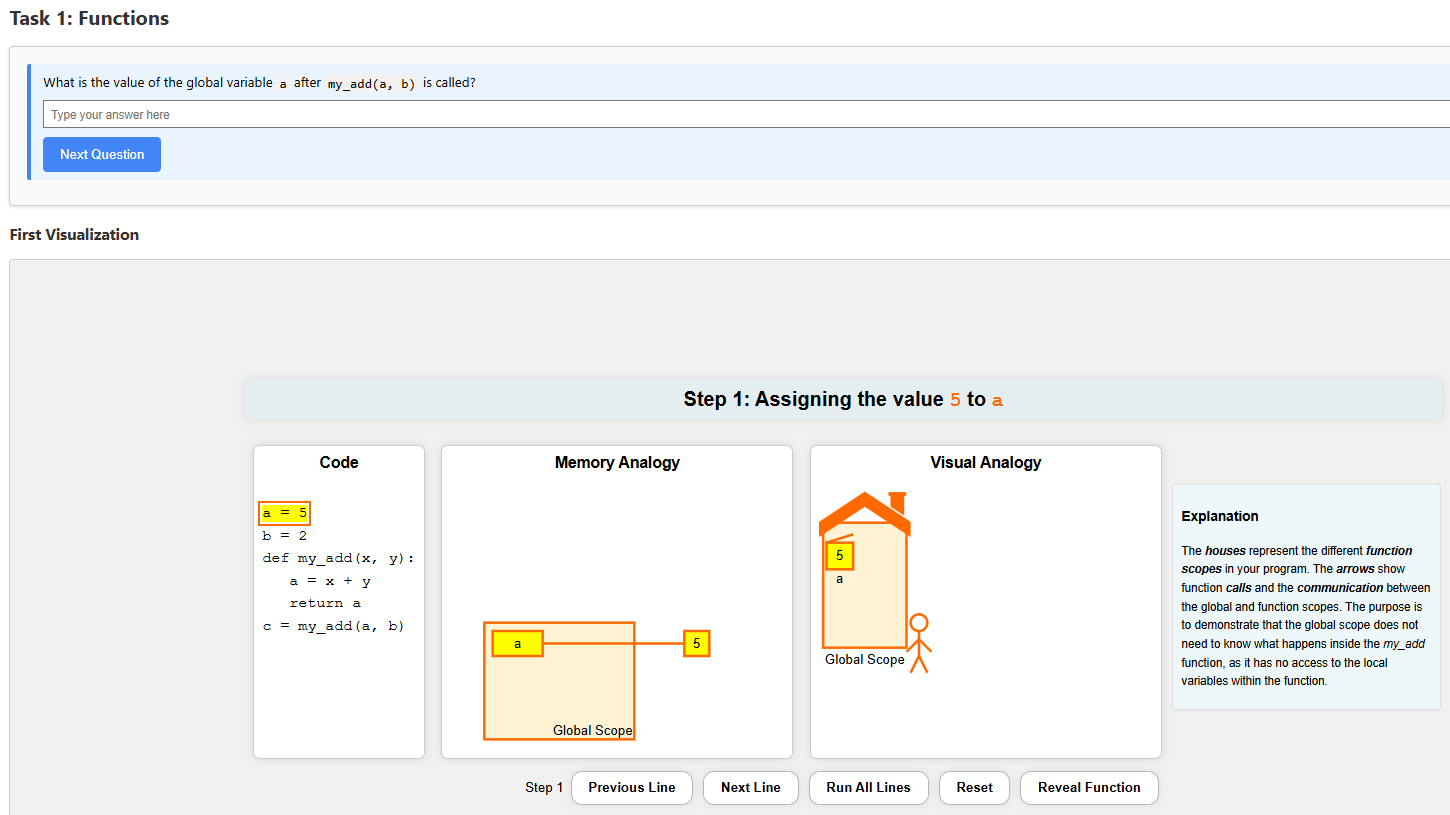}
    \caption{Multi-view visualization prototype}
    \label{fig:viz2}
\end{figure}

\appendix
\section{Appendix A: Minimal Gaze Processing Code}
\label{app:minimal-gaze}

\paragraph{Scope.}
Code below reproduces the reported gaze metrics: resampling to a fixed grid, AOI assignment (three-column interface), dwell times, AOI$\rightarrow$AOI transitions, and two diagnostic plots (transition matrix, AOI timeline). Extended analyses and exploratory figures are provided in our repository.

\begin{lstlisting}[language=Python,basicstyle=\ttfamily\small,breaklines=true]
import json
from dataclasses import dataclass
from typing import Dict, List, Optional, Tuple
import numpy as np, pandas as pd
import matplotlib.pyplot as plt

# ---- AOI model ----
@dataclass
class AOI:
    name: str; x0: int; y0: int; x1: int; y1: int
    def contains(self, x: float, y: float) -> bool:
        return (self.x0 <= x <= self.x1) and (self.y0 <= y <= self.y1)

# ---- Load combined JSON (eye/mouse arrays optional) ----
def load_combined_json(path: str):
    with open(path, "r") as f: data = json.load(f)
    eye   = pd.DataFrame(data.get("eyeTrackingData", []), columns=["elapsedTime","x","y"])
    mouse = pd.DataFrame(data.get("mouseTrackingData", []), columns=["elapsedTime","x","y"])
    for df in (eye, mouse):
        if not df.empty:
            df.sort_values("elapsedTime", inplace=True)
            df.reset_index(drop=True, inplace=True)
            df["elapsedTime"] -= df["elapsedTime"].min()
    return eye, mouse

# ---- Resample to fixed grid (e.g., 16 ms ~ 60 Hz) ----
def resample_stream(df: pd.DataFrame, freq_ms: int = 16, method: str = "nearest"):
    if df.empty: return df.copy()
    df2 = df.copy()
    df2["x"] = pd.to_numeric(df2["x"], errors="coerce")
    df2["y"] = pd.to_numeric(df2["y"], errors="coerce")
    df2["t"] = pd.to_timedelta(df2["elapsedTime"], unit="ms")
    df2 = df2.groupby("t")[["x","y"]].mean().sort_index()
    t0, t1 = df2.index.min(), df2.index.max()
    grid = pd.timedelta_range(start=t0, end=t1, freq=f"{freq_ms}ms")
    df2 = df2.reindex(df2.index.union(grid)).sort_index()
    if method == "nearest":
        df2["x"] = df2["x"].ffill().bfill()
        df2["y"] = df2["y"].ffill().bfill()
    else:
        df2["x"] = df2["x"].interpolate("time", limit_direction="both")
        df2["y"] = df2["y"].interpolate("time", limit_direction="both")
    out = df2.reindex(grid).reset_index(names="t")
    out["elapsedTime"] = (out["t"].dt.total_seconds() * 1000).astype(int)
    return out[["elapsedTime","x","y"]]

# ---- AOI assignment + metrics ----
def assign_aoi(df: pd.DataFrame, aois: Dict[str, AOI]) -> pd.DataFrame:
    names=[]
    for _, r in df.iterrows():
        name=None
        for a in aois.values():
            if a.contains(r["x"], r["y"]): name=a.name; break
        names.append(name)
    out=df.copy(); out["AOI"]=names; return out

def dwell_time_by_aoi(df: pd.DataFrame, time_col="elapsedTime"):
    if df.empty or "AOI" not in df: return pd.DataFrame(columns=["AOI","dwell_ms"])
    diffs=np.diff(df[time_col].values); dt=np.median(diffs) if len(diffs) else 0
    counts=df.groupby("AOI").size().rename("n").reset_index()
    counts["dwell_ms"]=counts["n"]*dt
    return counts[["AOI","dwell_ms"]].sort_values("dwell_ms", ascending=False)

def _aoi_runs(df: pd.DataFrame, time_col="elapsedTime")->List[dict]:
    if df.empty or "AOI" not in df: return []
    t=df[time_col].to_numpy(); a=df["AOI"].to_numpy(object)
    runs=[]; s=0
    for i in range(1,len(a)):
        if a[i]!=a[i-1]:
            runs.append({"aoi":a[s],"start":int(t[s]),"end":int(t[i-1]),"dur":int(t[i-1]-t[s])}); s=i
    runs.append({"aoi":a[s],"start":int(t[s]),"end":int(t[-1]),"dur":int(t[-1]-t[s])})
    return runs

def transition_matrix(df: pd.DataFrame, aois: Dict[str, AOI],
    *, time_col="elapsedTime", min_gap_ms=500, lag_ms=800, min_src_ms=100, min_dst_ms=150, count_self=False):
    runs=_aoi_runs(df,time_col); labels=[a.name for a in aois.values()]
    idx={n:i for i,n in enumerate(labels)}; mat=np.zeros((len(labels),len(labels)), int)
    def find_run_after(t_thresh:int)->Optional[int]:
        for j,r in enumerate(runs):
            if r["start"]<=t_thresh<=r["end"]: return j
        for j,r in enumerate(runs):
            if r["start"]>=t_thresh: return j
        return None
    for i in range(len(runs)-1):
        src=runs[i]
        if src["aoi"] is None or src["dur"]<min_src_ms: continue
        j=find_run_after(src["end"]+min_gap_ms+lag_ms)
        if j is None: continue
        dst=runs[j]
        if dst["aoi"] is None or dst["dur"]<min_dst_ms: continue
        if not count_self and dst["aoi"]==src["aoi"]: continue
        if src["aoi"] in idx and dst["aoi"] in idx:
            mat[idx[src["aoi"]], idx[dst["aoi"]]] += 1
    import pandas as pd
    return pd.DataFrame(mat, index=labels, columns=labels), labels

# ---- Infer 3-column AOIs (Code|Memory|Visual) or equal-thirds fallback ----
def infer_three_column_aois_from_gaze(gaze_df: pd.DataFrame, screen_size: Tuple[int,int],
    names=("Code","Memory","Visual"), pad_x=24, min_cluster_frac=0.03, full_height=True):
    W,H=screen_size
    if gaze_df.empty:
        thirds=[0,W//3,2*W//3,W]
        return {names[i]:(thirds[i],0,thirds[i+1],H) for i in range(3)}
    x=gaze_df["x"].to_numpy(float)
    centers=np.quantile(x,[0.17,0.5,0.83])
    for _ in range(30):
        d2=(x[:,None]-centers[None,:])**2; lab=d2.argmin(axis=1)
        new=centers.copy()
        for j in range(3):
            pts=x[lab==j]; 
            if pts.size: new[j]=pts.mean()
        if np.allclose(new,centers,atol=1e-3): break
        centers=new
    order=np.argsort(centers)
    counts=np.array([(lab==j).sum() for j in order])
    if (counts/ max(1,lab.size) < min_cluster_frac).any():
        thirds=[0,W//3,2*W//3,W]
        return {names[i]:(thirds[i],0,thirds[i+1],H) for i in range(3)}
    aois={}
    for name,j in zip(names,order):
        pts=gaze_df.loc[lab==j,["x","y"]].to_numpy(float)
        x0=int(max(0,np.floor(pts[:,0].min()-pad_x))); x1=int(min(W,np.ceil(pts[:,0].max()+pad_x)))
        y0,y1=(0,H) if full_height else (int(pts[:,1].min()), int(pts[:,1].max()))
        aois[name]=(x0,y0,x1,y1)
    return aois

# ---- Minimal figures (used in paper) ----
def plot_transition_matrix(dfm, outfile=None):
    plt.figure(figsize=(5,4)); plt.imshow(dfm.values, origin="upper", aspect="equal")
    plt.xticks(range(len(dfm.columns)), dfm.columns, rotation=45, ha="right")
    plt.yticks(range(len(dfm.index)), dfm.index); plt.colorbar(label="Transition count")
    plt.title("AOI Transition Matrix")
    if outfile: plt.savefig(outfile, dpi=200, bbox_inches="tight"); plt.close()
    else: plt.show()

def plot_aoi_timeline(df_with_aoi, aois: Dict[str, AOI], window_ms=250, outfile=None):
    if df_with_aoi.empty or "AOI" not in df_with_aoi: return
    t=df_with_aoi["elapsedTime"].to_numpy(); a=df_with_aoi["AOI"].to_numpy(object)
    windows=np.arange(int(t.min()), int(t.max())+window_ms, window_ms)
    labels=list(aois.keys()); idx={k:i for i,k in enumerate(labels)}
    from collections import Counter
    dom=[]; centers=[]
    for i in range(len(windows)-1):
        m=(t>=windows[i]) & (t<windows[i+1]); vals=[v for v in a[m] if v is not None]
        dom.append(idx[Counter(vals).most_common(1)[0][0]] if vals else np.nan)
        centers.append((windows[i]+windows[i+1])/2)
    plt.figure(figsize=(8,1.9)); plt.plot(centers, dom, linewidth=8)
    plt.yticks(range(len(labels)), labels); plt.xlabel("Time (ms)"); plt.title("Dominant AOI over time")
    if outfile: plt.savefig(outfile, dpi=200, bbox_inches="tight"); plt.close()
    else: plt.show()

# ---- Tiny driver (example) ----
if __name__ == "__main__":
    eye,_ = load_combined_json("path/to/tracking_data.json")
    eye_r = resample_stream(eye, 16)
    aois_rects = infer_three_column_aois_from_gaze(eye_r, (1280,720))
    aois_map = {n: AOI(n,*rect) for n,rect in aois_rects.items()}
    eye_aoi = assign_aoi(eye_r, aois_map)
    dwell = dwell_time_by_aoi(eye_aoi)
    tm,_ = transition_matrix(eye_aoi, aois_map)
    # optional figures used in paper:
    plot_transition_matrix(tm)
    plot_aoi_timeline(eye_aoi, aois_map)
\end{lstlisting}
