# Supplementary material for: Code as Anchor, Memory and Metaphor as Support: Learner Experiences with Multi-View Visualizations
Source: arXiv:2606.19570 source file (2026-06-17)
Supplement: Supplementary file 2 [file code.tex]

\appendix
\section{Appendix A: Minimal Gaze Processing Code}
\label{app:minimal-gaze}

\paragraph{Scope.}
Code below reproduces the reported gaze metrics: resampling to a fixed grid, AOI assignment (three-column interface), dwell times, AOI$\rightarrow$AOI transitions, and two diagnostic plots (transition matrix, AOI timeline). Extended analyses and exploratory figures are provided in our repository.

\begin{lstlisting}[language=Python,basicstyle=\ttfamily\small,breaklines=true]
import json
from dataclasses import dataclass
from typing import Dict, List, Optional, Tuple
import numpy as np, pandas as pd
import matplotlib.pyplot as plt

# ---- AOI model ----
@dataclass
class AOI:
    name: str; x0: int; y0: int; x1: int; y1: int
    def contains(self, x: float, y: float) -> bool:
        return (self.x0 <= x <= self.x1) and (self.y0 <= y <= self.y1)

# ---- Load combined JSON (eye/mouse arrays optional) ----
def load_combined_json(path: str):
    with open(path, "r") as f: data = json.load(f)
    eye   = pd.DataFrame(data.get("eyeTrackingData", []), columns=["elapsedTime","x","y"])
    mouse = pd.DataFrame(data.get("mouseTrackingData", []), columns=["elapsedTime","x","y"])
    for df in (eye, mouse):
        if not df.empty:
            df.sort_values("elapsedTime", inplace=True)
            df.reset_index(drop=True, inplace=True)
            df["elapsedTime"] -= df["elapsedTime"].min()
    return eye, mouse

# ---- Resample to fixed grid (e.g., 16 ms ~ 60 Hz) ----
def resample_stream(df: pd.DataFrame, freq_ms: int = 16, method: str = "nearest"):
    if df.empty: return df.copy()
    df2 = df.copy()
    df2["x"] = pd.to_numeric(df2["x"], errors="coerce")
    df2["y"] = pd.to_numeric(df2["y"], errors="coerce")
    df2["t"] = pd.to_timedelta(df2["elapsedTime"], unit="ms")
    df2 = df2.groupby("t")[["x","y"]].mean().sort_index()
    t0, t1 = df2.index.min(), df2.index.max()
    grid = pd.timedelta_range(start=t0, end=t1, freq=f"{freq_ms}ms")
    df2 = df2.reindex(df2.index.union(grid)).sort_index()
    if method == "nearest":
        df2["x"] = df2["x"].ffill().bfill()
        df2["y"] = df2["y"].ffill().bfill()
    else:
        df2["x"] = df2["x"].interpolate("time", limit_direction="both")
        df2["y"] = df2["y"].interpolate("time", limit_direction="both")
    out = df2.reindex(grid).reset_index(names="t")
    out["elapsedTime"] = (out["t"].dt.total_seconds() * 1000).astype(int)
    return out[["elapsedTime","x","y"]]

# ---- AOI assignment + metrics ----
def assign_aoi(df: pd.DataFrame, aois: Dict[str, AOI]) -> pd.DataFrame:
    names=[]
    for _, r in df.iterrows():
        name=None
        for a in aois.values():
            if a.contains(r["x"], r["y"]): name=a.name; break
        names.append(name)
    out=df.copy(); out["AOI"]=names; return out

def dwell_time_by_aoi(df: pd.DataFrame, time_col="elapsedTime"):
    if df.empty or "AOI" not in df: return pd.DataFrame(columns=["AOI","dwell_ms"])
    diffs=np.diff(df[time_col].values); dt=np.median(diffs) if len(diffs) else 0
    counts=df.groupby("AOI").size().rename("n").reset_index()
    counts["dwell_ms"]=counts["n"]*dt
    return counts[["AOI","dwell_ms"]].sort_values("dwell_ms", ascending=False)

def _aoi_runs(df: pd.DataFrame, time_col="elapsedTime")->List[dict]:
    if df.empty or "AOI" not in df: return []
    t=df[time_col].to_numpy(); a=df["AOI"].to_numpy(object)
    runs=[]; s=0
    for i in range(1,len(a)):
        if a[i]!=a[i-1]:
            runs.append({"aoi":a[s],"start":int(t[s]),"end":int(t[i-1]),"dur":int(t[i-1]-t[s])}); s=i
    runs.append({"aoi":a[s],"start":int(t[s]),"end":int(t[-1]),"dur":int(t[-1]-t[s])})
    return runs

def transition_matrix(df: pd.DataFrame, aois: Dict[str, AOI],
    *, time_col="elapsedTime", min_gap_ms=500, lag_ms=800, min_src_ms=100, min_dst_ms=150, count_self=False):
    runs=_aoi_runs(df,time_col); labels=[a.name for a in aois.values()]
    idx={n:i for i,n in enumerate(labels)}; mat=np.zeros((len(labels),len(labels)), int)
    def find_run_after(t_thresh:int)->Optional[int]:
        for j,r in enumerate(runs):
            if r["start"]<=t_thresh<=r["end"]: return j
        for j,r in enumerate(runs):
            if r["start"]>=t_thresh: return j
        return None
    for i in range(len(runs)-1):
        src=runs[i]
        if src["aoi"] is None or src["dur"]<min_src_ms: continue
        j=find_run_after(src["end"]+min_gap_ms+lag_ms)
        if j is None: continue
        dst=runs[j]
        if dst["aoi"] is None or dst["dur"]<min_dst_ms: continue
        if not count_self and dst["aoi"]==src["aoi"]: continue
        if src["aoi"] in idx and dst["aoi"] in idx:
            mat[idx[src["aoi"]], idx[dst["aoi"]]] += 1
    import pandas as pd
    return pd.DataFrame(mat, index=labels, columns=labels), labels

# ---- Infer 3-column AOIs (Code|Memory|Visual) or equal-thirds fallback ----
def infer_three_column_aois_from_gaze(gaze_df: pd.DataFrame, screen_size: Tuple[int,int],
    names=("Code","Memory","Visual"), pad_x=24, min_cluster_frac=0.03, full_height=True):
    W,H=screen_size
    if gaze_df.empty:
        thirds=[0,W//3,2*W//3,W]
        return {names[i]:(thirds[i],0,thirds[i+1],H) for i in range(3)}
    x=gaze_df["x"].to_numpy(float)
    centers=np.quantile(x,[0.17,0.5,0.83])
    for _ in range(30):
        d2=(x[:,None]-centers[None,:])**2; lab=d2.argmin(axis=1)
        new=centers.copy()
        for j in range(3):
            pts=x[lab==j]; 
            if pts.size: new[j]=pts.mean()
        if np.allclose(new,centers,atol=1e-3): break
        centers=new
    order=np.argsort(centers)
    counts=np.array([(lab==j).sum() for j in order])
    if (counts/ max(1,lab.size) < min_cluster_frac).any():
        thirds=[0,W//3,2*W//3,W]
        return {names[i]:(thirds[i],0,thirds[i+1],H) for i in range(3)}
    aois={}
    for name,j in zip(names,order):
        pts=gaze_df.loc[lab==j,["x","y"]].to_numpy(float)
        x0=int(max(0,np.floor(pts[:,0].min()-pad_x))); x1=int(min(W,np.ceil(pts[:,0].max()+pad_x)))
        y0,y1=(0,H) if full_height else (int(pts[:,1].min()), int(pts[:,1].max()))
        aois[name]=(x0,y0,x1,y1)
    return aois

# ---- Minimal figures (used in paper) ----
def plot_transition_matrix(dfm, outfile=None):
    plt.figure(figsize=(5,4)); plt.imshow(dfm.values, origin="upper", aspect="equal")
    plt.xticks(range(len(dfm.columns)), dfm.columns, rotation=45, ha="right")
    plt.yticks(range(len(dfm.index)), dfm.index); plt.colorbar(label="Transition count")
    plt.title("AOI Transition Matrix")
    if outfile: plt.savefig(outfile, dpi=200, bbox_inches="tight"); plt.close()
    else: plt.show()

def plot_aoi_timeline(df_with_aoi, aois: Dict[str, AOI], window_ms=250, outfile=None):
    if df_with_aoi.empty or "AOI" not in df_with_aoi: return
    t=df_with_aoi["elapsedTime"].to_numpy(); a=df_with_aoi["AOI"].to_numpy(object)
    windows=np.arange(int(t.min()), int(t.max())+window_ms, window_ms)
    labels=list(aois.keys()); idx={k:i for i,k in enumerate(labels)}
    from collections import Counter
    dom=[]; centers=[]
    for i in range(len(windows)-1):
        m=(t>=windows[i]) & (t<windows[i+1]); vals=[v for v in a[m] if v is not None]
        dom.append(idx[Counter(vals).most_common(1)[0][0]] if vals else np.nan)
        centers.append((windows[i]+windows[i+1])/2)
    plt.figure(figsize=(8,1.9)); plt.plot(centers, dom, linewidth=8)
    plt.yticks(range(len(labels)), labels); plt.xlabel("Time (ms)"); plt.title("Dominant AOI over time")
    if outfile: plt.savefig(outfile, dpi=200, bbox_inches="tight"); plt.close()
    else: plt.show()

# ---- Tiny driver (example) ----
if __name__ == "__main__":
    eye,_ = load_combined_json("path/to/tracking_data.json")
    eye_r = resample_stream(eye, 16)
    aois_rects = infer_three_column_aois_from_gaze(eye_r, (1280,720))
    aois_map = {n: AOI(n,*rect) for n,rect in aois_rects.items()}
    eye_aoi = assign_aoi(eye_r, aois_map)
    dwell = dwell_time_by_aoi(eye_aoi)
    tm,_ = transition_matrix(eye_aoi, aois_map)
    # optional figures used in paper:
    plot_transition_matrix(tm)
    plot_aoi_timeline(eye_aoi, aois_map)
\end{lstlisting}
