# Supplementary material for: Code as Anchor, Memory and Metaphor as Support: Learner Experiences with Multi-View Visualizations
Source: arXiv:2606.19570 source file (2026-06-17)
Supplement: Supplementary file 3 [file interview-protocol.tex]

\begin{tcolorbox}[colback=gray!5,colframe=black!40,arc=3mm,boxrule=0.5pt]

\subsection*{General Guidelines}

\paragraph{Introduction.} 
Explain the purpose of the study, obtain consent, and collect brief demographic information (programming experience, language background, etc.).

\paragraph{Think-Aloud Protocol.} 
Remind participants to verbalize their thoughts as they work through the visual examples. Encourage them to describe what they see, what they think is happening, and any challenges they face.

\paragraph{Observations.} 
Make brief notes on any points of confusion, hesitation, or interesting comments that arise during the tasks.
\end{tcolorbox}

\begin{tcolorbox}[colback=gray!5,colframe=black!40,arc=3mm,boxrule=0.5pt]
\subsection*{Group-Specific Instructions}

\paragraph{Group A.} TOOL LINK REDACTED

\paragraph{Group B.} TOOL LINK REDACTED

\paragraph{Tool Sequence Introduction.} 
Inform the participant: 
\begin{quote}
``Today you will start with Python Tutor/MER tool. Once you complete each task with Python Tutor, you will switch to the MER tool/Python Tutor to complete the next task.''
\end{quote}

\paragraph{During Each Task.} 
Prompt the participant to follow along with the visual example. Ask:
\begin{itemize}
    \item What do you notice in this visual representation?
    \item How is the change in variables or control flow depicted for you?
\end{itemize}

\paragraph{Task-Specific Follow-Up Questions.}
\begin{itemize}
    \item \textbf{Task 1: Functions} --- ``What part of the visualization clarified function scope for you?''
    \item \textbf{Task 2: While Loops} --- ``As you followed the while loop, what visual cues helped you see the progression of the counter?'' ``Were there any parts of the loop’s execution that you felt needed more clarity?''
    \item \textbf{Task 3: Linked List} --- ``What did you observe about how the linked list structure changed after the append operation?''
\end{itemize}

\paragraph{Transition Questions (After Completing the First Tool).}
\begin{itemize}
    \item How would you compare your understanding of the tasks after using Python Tutor?
    \item Are there any aspects you found particularly helpful or limiting in Python Tutor before you switch to the next tool?
\end{itemize}

\paragraph{After the Second Tool (MER Tool).} 
Ask similar follow-up questions, encouraging comparisons:
\begin{itemize}
    \item What differences do you notice between Python Tutor and the MER Tool?
    \item Which tool provided clearer visual cues for you, and why?
    \item Were there any moments in the MER/PT Tool where the visualization significantly changed your understanding of the code?
\end{itemize}
\end{tcolorbox}

\begin{tcolorbox}[colback=gray!5,colframe=black!40,arc=3mm,boxrule=0.5pt]

\subsection*{Post-Task Interview}

\paragraph{Overall Tool Effectiveness.}
\begin{itemize}
    \item Overall, which tool did you find more helpful for understanding the programming concepts? Why?
    \item Were there any specific visual features in one tool that you preferred over the other?
\end{itemize}

\paragraph{Usability and Cognitive Load.}
\begin{itemize}
    \item How easy was it to follow the code execution in each tool?
    \item Did you feel that any of the visualizations were overwhelming or confusing at any point?
\end{itemize}

\paragraph{Suggestions for Improvement.}
\begin{itemize}
    \item If you could improve one aspect of either tool’s visualization, what would it be?
    \item Do you have any suggestions for making the visualizations more intuitive or informative?
\end{itemize}

\paragraph{Final Thoughts.} 
\begin{itemize}
    \item Is there anything else you’d like to share about your experience with these tools?
\end{itemize}
\end{tcolorbox}

\begin{tcolorbox}[colback=gray!5,colframe=black!40,arc=3mm,boxrule=0.5pt]

\subsection*{Closing the Session}

Thank the participant for their time and contributions. Remind them about data confidentiality and any follow-up procedures.  

\end{tcolorbox}
