# Supplementary material for: Code as Anchor, Memory and Metaphor as Support: Learner Experiences with Multi-View Visualizations
Source: arXiv:2606.19570 source file (2026-06-17)
Supplement: Supplementary file 4 [file recruitment.tex]

\section{Recruitment Emails (Anonymized)}
\label{recruit-email}

\begin{tcolorbox}[colback=gray!5,colframe=black!40,arc=3mm,boxrule=0.5pt]
\textbf{Subject:} Share Your Thoughts on Programming Tools and Earn a \$30 Gift Card  

\vspace{1em}
Dear [Student Name],  

\vspace{0.5em}
We are conducting a research study to understand how visual analogy programming tools can help students learn programming concepts. As a former [introductory programming course] student, your experiences and feedback would be invaluable to this study!  

\vspace{0.5em}
The study involves a 45--60 minute in-person interview where you will:  
\begin{itemize}
    \item Discuss your experiences with programming tools.  
    \item Share your thoughts on visual representations of programming concepts like functions, conditions, lists, and sorting.  
    \item Help us identify ways to improve these tools for future learners.  
\end{itemize}

As a thank-you, participants will receive a \$30 gift card after completing the interview.  

\vspace{0.5em}
If you’re interested, please reply to this email or fill out [form link] by [deadline, if applicable]. We’ll reach out to schedule a time that works for you.  

\vspace{0.5em}
Thank you for considering this opportunity!  

\vspace{1em}
Best regards,  \\
Researcher Name \\ 
Position/Role \\
Institution Name \\
\end{tcolorbox}
