# Supplementary material for: Code as Anchor, Memory and Metaphor as Support: Learner Experiences with Multi-View Visualizations
Source: arXiv:2606.19570 source file (2026-06-17)
Supplement: Supplementary file 5 [file tasks.tex]

\begin{table}[h]
\centering

\begin{tabular}{|p{2.5cm}|p{9.5cm}|p{3cm}|}
\hline
\textbf{Topic} & \textbf{Question} & \textbf{Type} \\
\hline
\multirow{3}{*}{\textbf{Scope}} 
& What is the value of the global variable \texttt{a} after \texttt{my\_add(a, b)} is called? & Tracing \\
\cline{2-3}
& What is the value of the local variable \texttt{a} right before the return statement? & Tracing \\
\cline{2-3}
& Explain why the global variable remains unchanged. & Explaining \\
\hline
\multirow{3}{*}{\textbf{While Loops}} 
& What value will be printed? Trace each step of the loop. & Tracing \\
\cline{2-3}
& Explain in plain English how the while loop searches for the item. What role does the counter play, and how does the loop stop? & Explaining \\
\cline{2-3}
& How would you modify the code so that if the wanted item is not in the list, the program prints ``Item not found'' instead of running indefinitely? & Extending \\
\hline
\multirow{3}{*}{\textbf{Linked Lists}} 
& What are the values of \texttt{data} and \texttt{next} for each node in the list? List them in order. & Tracing \\
\cline{2-3}
& Explain how the append function works when adding a new node, differentiating between an empty list and a populated list. & Explaining \\
\cline{2-3}
& How would you implement a \texttt{find(data)} method, and what would happen if the value does not exist? & Extending \\
\hline
\end{tabular}
\caption{Student task questions organized by topic and type.}
\label{tab:student-task-questions}
\end{table}
